# Supplementary material for: MobileAtlas: Geographically Decoupled Measurements in Cellular Networks for Security and Privacy Research
Source: arXiv:2403.08507 source file (2024-03-13)
Supplement: Supplementary file 1 [file USENIX-23-Artifact-Appendix-MobileAtlas.pdf]

# USENIX'23 Artifact Appendix:

## MOBILEATLAS: Geographically Decoupled Measurements in Cellular Networks for Security and Privacy Research

Gabriel K. Gegenhuber  
University of Vienna\*

Wilfried Mayer  
SBA Research

Edgar Weippl  
University of Vienna

Adrian Dabrowski  
CISPA Helmholtz Center for Information Security†

### A Artifact Appendix

MOBILEATLAS is a scalable, cost-efficient test framework for cellular networks that takes international roaming measurements to the next level. It implements the promising approach to geographically decouple SIM card and modem, which boosts the scalability and flexibility of the measurement platform. It offers versatile capabilities and a controlled environment that makes a good foundation for qualitative and fine-grained cellular measurements.

#### A.1 Abstract

Physically moving devices and SIM cards between countries to enable measurements in a roaming environment is costly and does not scale well. Therefore, we introduce an approach to geographically detach the SIM card from the modem by tunneling the SIM card's protocol over the Internet and emulating its signal on the cellular modem. This allows us to test roaming effects on a large number of operators without physically moving any hardware between different countries.

To make it accessible to other researchers, we fully release the hard- and software documentation of our measurement framework.

#### A.2 Description & Requirements

##### A.2.1 Security, privacy, and ethical concerns

MOBILEATLAS is meant to be used in live mobile networks. Our measurement experiments usually mimic normal user behavior and just transmit minimal data traffic (i.e., several MB of data) to get deeper insights into the operator's core network mechanisms and interplay during roaming scenarios. However, due to SIM tunneling, SIM cards could change the "country" in an irregular and fast fashion, which might spark

confusion among the operator's systems or trigger fraud control alerts. In order to exercise caution, we manually imposed a waiting time of 2 hours between country switches in our experiments. When testing for potential free-riding possibilities, we always made sure not to enrich ourselves by not oversizing the generated test traffic and by letting an equal or greater amount of our monthly traffic allowance expire at the end of the month (as if we were billed for the traffic).

##### A.2.2 How to access

The hard- and software documentation of the MOBILEATLAS measurement platform that is presented in our paper is hosted on [GitHub](#).

##### A.2.3 Hardware dependencies

*SIM Providers* require a host system (e.g., a linux laptop), a SIM reader device (e.g., PC/SC reader) and a SIM card that will be made accessible (i.e., to an external *Measurement Probe* via a SIM tunnel).

*Measurement Probes* require a dedicated hardware setup. To support future upgrades, most of the used hardware components are easily interchangeable. We based our current probe version on a Raspberry Pi 4 and a Quectel EG25G modem. Furthermore, we use a HAT adapter to connect the modem to the Pi. To tunnel and emulate the SIM card protocol we leverage the Pi's GPIO ports and connect them to the modems SIM socket via a [self-made SIM PCB](#).

More details and some pictures of the used hardware can be found on GitHub in a dedicated [README file](#).

##### A.2.4 Software dependencies

Our python-based source code relies on external dependencies that need to be installed via the package manager or via pip (cf. Section [A.3](#)). Besides common and officially available python

\* Supported by the UniVie Doctoral School Computer Science DoCS.

† Partly as postdoc at University of California, Irvine.

packages, we also require a customized version of [pySIM](#).

Furthermore, we use ModemManager <sup>1</sup> to interact with the modem during measurement experiments. Therefore, good ModemManager support is essential when using different hardware (i.e., a different modem) for the *Measurement Probe*.

#### A.2.5 Benchmarks

None

### A.3 Set-up

#### A.3.1 Installation

We use Ansible to patch and setup the system of our *Measurement Probes*. The Ansible playbooks are meant to be executed on a fresh installation of the Raspberry Pi OS, as described in a dedicated [README file](#).

The software dependencies that are needed for the *SIM Provider* are referenced in the next section.

#### A.3.2 Basic Test

To run the *SIM Provider* and *Measurement Probe* software components it is required to setup a Python virtual-environment as described in the responsible [README file](#).

### A.4 Version

Based on the LaTeX template for Artifact Evaluation V20220926. Submission, reviewing and badging methodology followed for the evaluation of this artifact can be found at <https://secartifacts.github.io/usenixsec2023/>.

---

<sup>1</sup><https://modemmanager.org/>
